# Supplementary material for: Floquet Non-Abelian Topological Insulator and Multifold Bulk-Edge Correspondence
Source: arXiv:2310.08819 source file (2023-10-13)

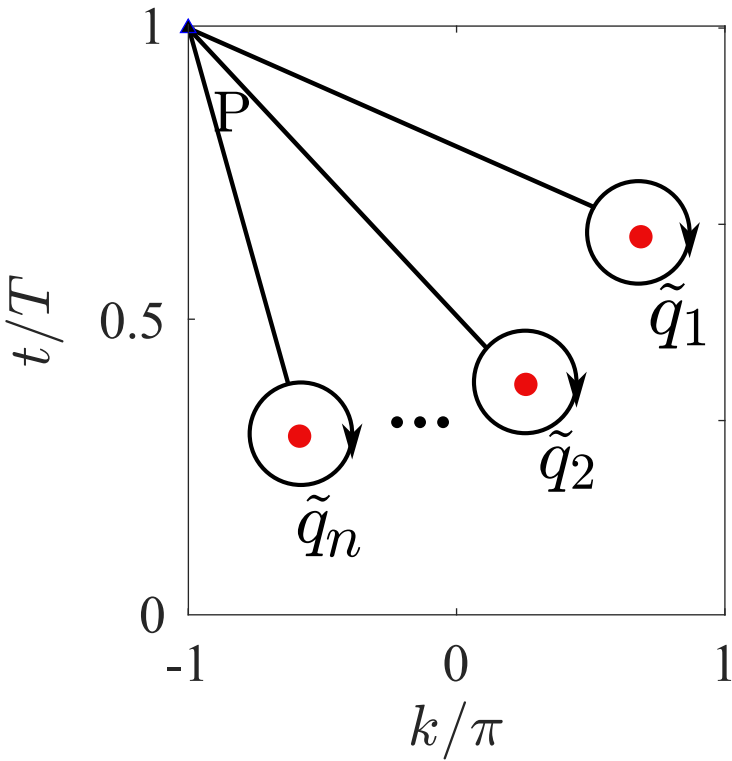

Supplement: Supplementary file 1 [file supp1.pdf]
